# Supplementary material for: Atom: Low-bit Quantization for Efficient and Accurate LLM Serving
Source: arXiv:2310.19102 source file (2024-04-16)
Supplement: Supplementary file 1 [file 10_Appendix.tex]

\section{Appendix}
